# Supplementary material for: Fidelity benchmarks for two-qubit gates in silicon
Source: arXiv:1805.05027 ancillary file (2018-07-27)
Supplement: Supplementary file 1 [file Supp.pdf]

## I. ENERGY SPECTRUM

Electrical detuning of the quantum dots via their top gate voltages $V_{\mathrm{G1}}$ and $V_{\mathrm{G2}}$ modifies their resonance frequencies via the Stark shift, and the exchange coupling by changing the energy gap between the (1,1) and (2,0) (Fig. S1) or (1,1) and (0,2) (Fig. S2) charge states. The Stark shift dominates the changes in resonance frequency deep inside the (1,1) regime and allows $\Delta E_Z/h$, the difference in Zeeman splitting of the qubits, to be adjusted by approximately 2 MHz using G1 and G2. When approaching the doubly-occupied charge state, two-qubit interaction becomes the main contributor to the curvature of the resonance frequency.

## II. SPIN TRANSPORT READOUT AND ERRORS

Spin relaxation hot-spots in the double quantum dot system[1] are measured at the (0,1)-(1,0) anti-crossing with a $|\uparrow\rangle$ relaxation time of $T_1 = 12 \pm 5$ µs (Fig. S3). While the spin life-time in the MOS quantum dots at 1.4 T is typically larger than 1 second[2], the hot-spot provides an alternative way for fast initialization. In the experiment, we stay at the hot-spot for 300 µs to ensure Q1 is initialized as $|\downarrow\rangle$ after the readout process.

## III. THEORETICAL DESCRIPTION OF THE SYSTEM

When the qubits in the (1,1) charge region are far detuned from a doubly-occupied charge state ((2,0) or (0,2)), the Hamiltonian in the two spin basis $(\uparrow\uparrow, \uparrow\downarrow, \downarrow\uparrow, \downarrow\downarrow)$ can be approximated as [3]

$$H = \frac{1}{2}\begin{pmatrix} 2\bar{E}_z & \gamma_2 B_1 & \gamma_1 B_1 & 0 \\ \gamma_2 B_1^* & \delta E_z - J & J & \gamma_1 B_1 \\ \gamma_1 B_1^* & J & -\delta E_z - J & \gamma_2 B_1 \\ 0 & \gamma_1 B_1^* & \gamma_2 B_1^* & -2\bar{E}_z \end{pmatrix}. \quad (1)$$

In order to be directly accessible by microwave, the Hamiltonian can be diagonalized into

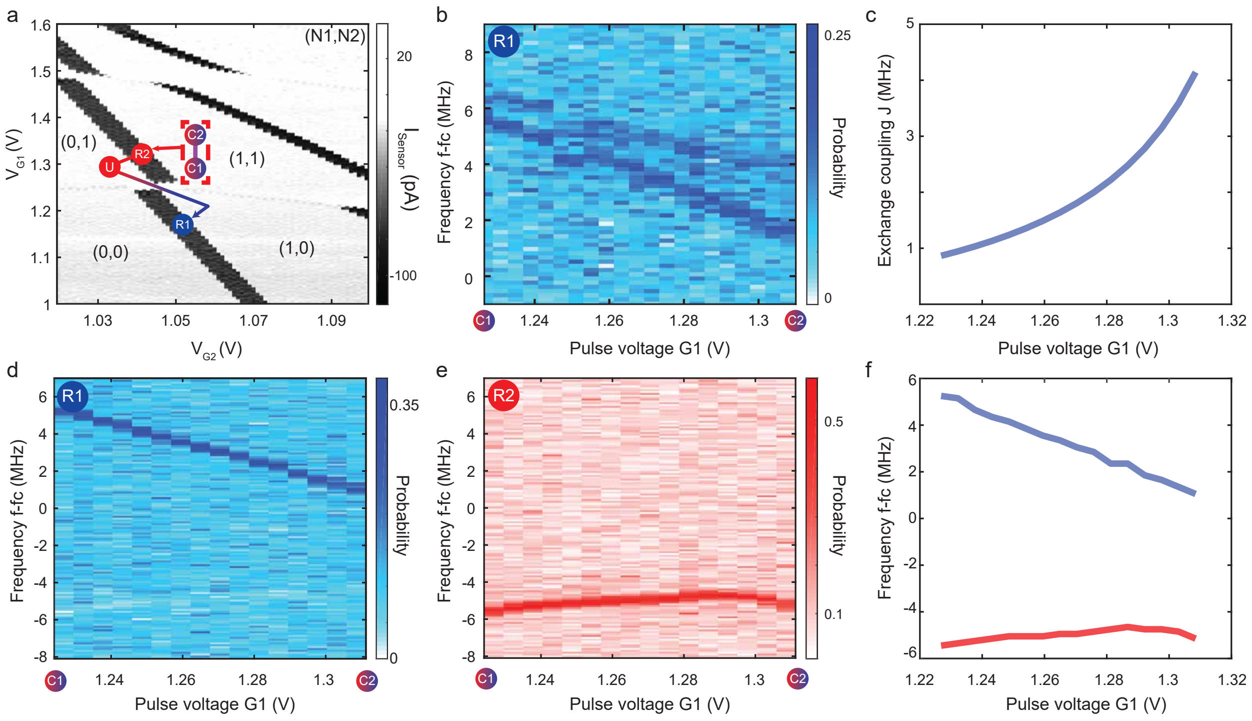


**Figure S1 | Energy and exchange spectrum as a function of $V_{\mathbf{G1}}$.** **(a)** Pulse sequence to measure the energy and exchange spectrum overlaid with the charge stability diagram. In the experiment, the control point is scanned from C1 to C2 to measure the change in ESR frequencies. **(b-c)** A $\frac{1}{\sqrt{2}}(|\tilde{\downarrow\uparrow}\rangle + |\downarrow\downarrow\rangle)$ state is prepared using ESR. The resonance frequency for Q1 is split into two branches $f_{1\downarrow}$ and $f_{1\uparrow}$ by exchange coupling as the control point approaches the (1,1)-(0,2) anti-crossing. The extracted frequency difference between $f_{1\downarrow}$ and $f_{1\uparrow}$ as a function of G1 voltage is plotted in (c). **(d-f)** Resonance spectrum when the system is initialized into the $|\downarrow\downarrow\rangle$ ground state. The resonance signal corresponding to $f_{1\downarrow}$ as a function of top gate voltage $V_{G1}$ is presented in (d) and the signal for the $f_{2\downarrow}$ transition in (e). **(f)** Extracted resonance frequency change for $f_{1\downarrow}$ and $f_{2\downarrow}$ due to G1 voltage.

the new basis $(\uparrow\uparrow, \tilde{\uparrow\downarrow}, \tilde{\downarrow\uparrow}, \downarrow\downarrow)$:

$$H = \frac{1}{2}\begin{pmatrix} 2\bar{E}_z & \gamma_{2\uparrow}B_1 & \gamma_{1\uparrow}B_1 & 0 \\ \gamma_{2\uparrow}B_1^* & \delta\tilde{E}_z - J & 0 & \gamma_{1\downarrow}B_1 \\ \gamma_{1\uparrow}B_1^* & 0 & -\delta\tilde{E}_z - J & \gamma_{2\downarrow}B_1 \\ 0 & \gamma_{1\downarrow}B_1^* & \gamma_{2\downarrow}B_1^* & -2\bar{E}_z \end{pmatrix}, \quad (2)$$

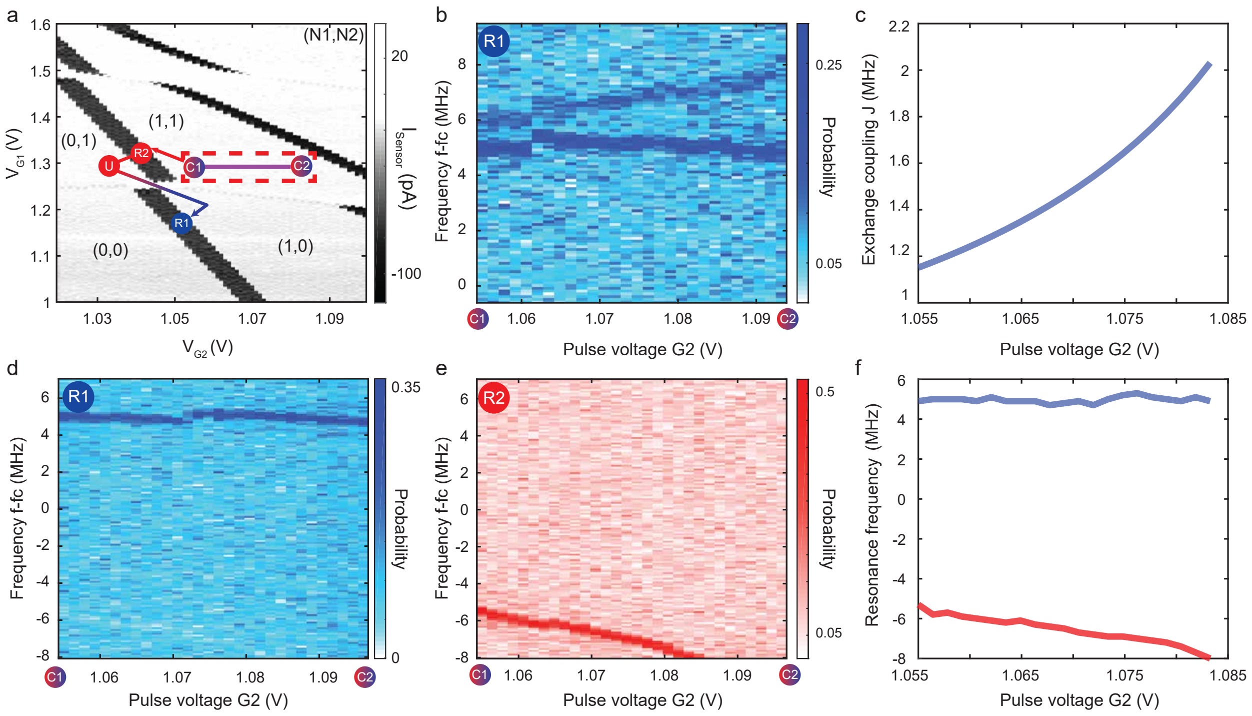


**Figure S2 | Energy and exchange spectrum as a function of $V_{\mathbf{G2}}$** All measurements are performed analogously to the ones presented in Fig. S1.

where $\tilde{E}_z = \sqrt{J^2 + \delta E_z^2}$, and

$$
\begin{aligned}
|\widetilde{\downarrow\uparrow}\rangle &= \cos\tfrac{\theta}{2}|\downarrow\uparrow\rangle + \sin\tfrac{\theta}{2}|\uparrow\downarrow\rangle \\
|\widetilde{\uparrow\downarrow}\rangle &= -\sin\tfrac{\theta}{2}|\downarrow\uparrow\rangle + \cos\tfrac{\theta}{2}|\uparrow\downarrow\rangle
\end{aligned}
. \qquad (3)
$$

Here, $\cos\frac{\theta}{2} = \frac{\delta E_z + \sqrt{J^2+\delta E_z^2}}{\sqrt{(\delta E_z + \sqrt{J^2+\delta E_z^2})^2 + J^2}}$ and $\sin\frac{\theta}{2} = \frac{J}{\sqrt{(\delta E_z + \sqrt{J^2+\delta E_z^2})^2 + J^2}}$, and thus the effective gyromagnetic ratios follow the rotation

$$
\begin{aligned}
\gamma_{1\uparrow} &= \gamma_1 \cos\tfrac{\theta}{2} - \gamma_2 \sin\tfrac{\theta}{2} \\
\gamma_{1\downarrow} &= \gamma_1 \cos\tfrac{\theta}{2} + \gamma_2 \sin\tfrac{\theta}{2} \\
\gamma_{2\uparrow} &= \gamma_2 \cos\tfrac{\theta}{2} + \gamma_1 \sin\tfrac{\theta}{2} \\
\gamma_{2\downarrow} &= \gamma_2 \cos\tfrac{\theta}{2} - \gamma_1 \sin\tfrac{\theta}{2}
\end{aligned}
. \qquad (4)
$$

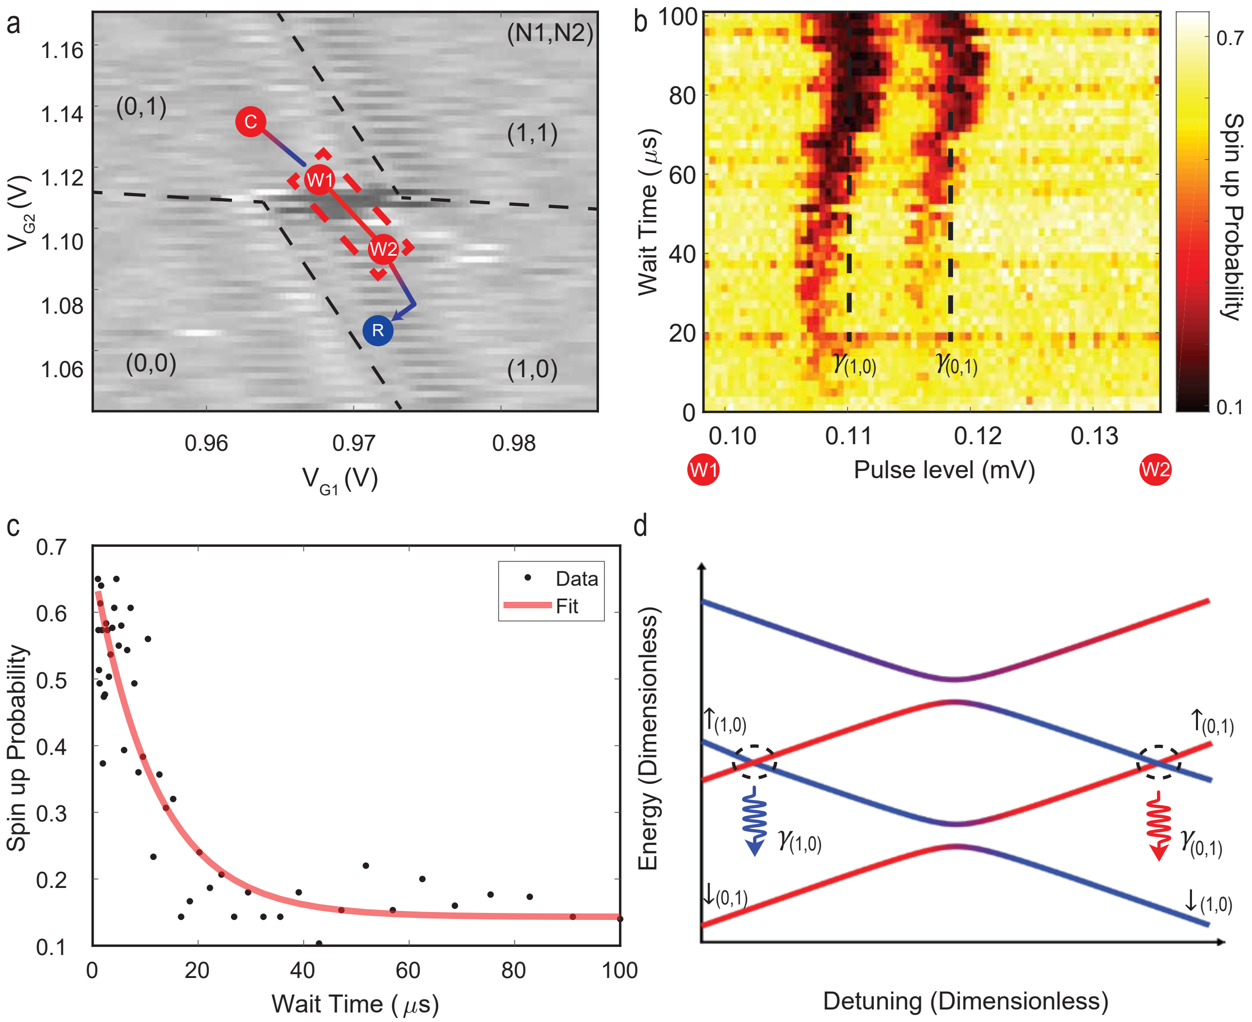


**Figure S3 | Hot-spot Relaxation (a)** The sequence to measure hot-spot relaxation overlaid with the stability diagram. The electron spin is prepared in the $|\uparrow\rangle$ state by an ESR $\pi$-pulse in the (0,1) region (point C). An adiabatic 1 μs voltage pulse then brings the spin to point W (between W1 and W2) for a wait time $\tau_w$. The state of the spin is later transferred to (1,0) region with another adiabatic 1 μs pulse, and then read via the (1,0)-(0,0) transition. **(b)** Spin-up probability as a function of wait time $\tau_w$ at different wait points W, varied from W1 to W2. Two spin relaxation hot-spots show up as regions with highly reduced spin-up probability. **(c)** Spin relaxation for the left hot-spot in (b). $T_1$ time for the hot spot is $12 \pm 5$ μs. **(d)** Schematic of the double quantum dot energy diagram around the (0,1)-(1,0) anti-crossing. The red lines represent the spin states in (0,1) region and the blue lines represent the spin states in (1,0) region.

The four resonance frequencies are:

$$\begin{aligned} f_{1\uparrow} &= \bar{E}_z + \tfrac{\delta\tilde{E}_z + J}{2} \\ f_{1\downarrow} &= \bar{E}_z + \tfrac{\delta\tilde{E}_z - J}{2} \\ f_{2\uparrow} &= \bar{E}_z + \tfrac{-\delta\tilde{E}_z + J}{2} \\ f_{2\downarrow} &= \bar{E}_z + \tfrac{-\delta\tilde{E}_z - J}{2} \end{aligned} . \tag{5}$$

To perform resonance operations, it is more convenient to describe the system in a time-dependent frame $H_{\rm RWA} = RHR^\dagger - i\frac{\partial R}{\partial t}R^\dagger$, with a rotating matrix $R$ =diag $\{e^{-i\bar{E}_z t}$, $e^{-i(\delta\tilde{E}_z - J)t}$, $e^{i(\delta\tilde{E}_z + J)t}$, $e^{i\bar{E}_z t}\}$. Microwave pulses on one selected frequency $f_{1\downarrow}$, $f_{1\uparrow}$, $f_{2\downarrow}$, $f_{2\uparrow}$ will result in a conditional rotation. Here, we take the Hamiltonian in the time-dependent frame with excitation frequency $f_{1\downarrow}$ when $B_1(t) = \frac{\Omega}{\gamma_{1\downarrow}}e^{if_{1\downarrow}t}$ as an example. After neglecting the far off-resonance terms, the Hamiltonian in the time-dependent frame can be written as

$$H_{\rm RWA} = \frac{\hbar}{2}\begin{pmatrix} 0 & 0 & 0 & 0 \\ 0 & 0 & 0 & \Omega \\ 0 & 0 & 0 & 0 \\ 0 & \Omega^* & 0 & 0 \end{pmatrix} + \frac{\hbar}{2}\frac{\gamma_{1\uparrow}}{\gamma_{1\downarrow}}\begin{pmatrix} 0 & 0 & \Omega e^{-iJt} & 0 \\ 0 & 0 & 0 & 0 \\ \Omega^* e^{iJt} & 0 & 0 & 0 \\ 0 & 0 & 0 & 0 \end{pmatrix} . \tag{6}$$

The time evolution of the first term yields the conditional rotation operator $U_{1\downarrow}$. However, the second term will result in a finite rotation and phase shift at the frequency $f_{1\uparrow}$, representing crosstalk between qubit states. In simulations, we find this crosstalk would contribute 7% of infidelity to the Clifford gates for our experimental parameters J=1.59 MHz and Ω=410 kHz. To cancel out the crosstalk error, the lengths and amplitudes of all conditional $\pi/2$-pulses are chosen such that the off-diagonal component of the second term is 0 after a $\pi/2$-pulse. We find that the length of the $\pi/2$-pulses must satisfy :

$$T_{\pi/2} = \frac{1}{8\Omega} = \frac{h\sqrt{16n^2 - \frac{\gamma_{1\uparrow}}{\gamma_{1\downarrow}}}}{4J} \approx \frac{h\sqrt{16n^2 - 1}}{4J}, \text{ where } n \geq 1. \tag{7}$$

In the experiment, we choose the shortest possible conditional $\pi/2$ length at the given microwave power to avoid dephasing. The phase error caused by off-resonance drive is corrected by compensating the phase in future pulses of a particular frequency[4].

In order to achieve a single qubit operation, two sequential pulses were put in sequence $B_1(t) = \frac{\Omega}{\gamma_{1\downarrow}} e^{if_{1\downarrow}t}\Theta(0)[1-\Theta(t_\pi)] + \frac{\Omega}{\gamma_{1\uparrow}} e^{if_{1\uparrow}t}\Theta(t_\pi)[1-\Theta(2t_\pi)]$. Here, $\Theta(t)$ is the Heaviside function. Since the microwave drive controls both the rotation and the rotation axis, two-axis control is performed by adapting the rotation axis with the IQ mixer in the microwave source[5] by applying a phase offset to future pulses. This is equivalent to a Z-rotation on a specific transitions.

## IV. QUASI-STATIC DETUNING NOISE

To estimate the errors in the randomized benchmarking experiment, we import the pulse sequences from randomized benchmarking sequences into a time evolution simulator. The simulation calculates the operator at any specific time $U_{dt}(t) = e^{-iH(t)dt}$, resulting in a final operator $U = \prod_{t=te}^{t=ti} U_{dt}(t)$. Random Clifford sequences of length $L$ are averaged over multiple runs until the projected state probability as a function of $L$ resembles an exponential decay. We fit $P = A(1-\frac{4}{3}r_c) + B$ to the decay curve and obtained the Clifford gate fidelity of $F_c = 1-r_c$. We simulate the Clifford sequence including the crosstalk correction as described in the previous section and with no charge noise components, and obtain $F_{\text{Clifford}} > 99.9$ %.

The effect of stochastic noise is introduced into the model by Hamiltonian fluctuations on all four levels. The Hamiltonian can be described by:

$$\delta H = h \begin{pmatrix} \delta f_{\uparrow\uparrow} & 0 & 0 & 0 \\ 0 & \delta f_{\uparrow\downarrow} & 0 & 0 \\ 0 & 0 & \delta f_{\downarrow\uparrow} & 0 \\ 0 & 0 & 0 & \delta f_{\downarrow\downarrow} \end{pmatrix}. \tag{8}$$

However, since only 3 of the fluctuation terms are independent, we choose $\delta f_{\downarrow\downarrow} = 0$ for simplicity. To obtain the stochastic noise for each level, we measured free induction decay for different superposition states: $T^*_{2,1\downarrow} = 24.3 \pm 2$ µs, $T^*_{2,1\uparrow} = 8.6 \pm 1$ µs, $T^*_{2,2\downarrow} = 10.5 \pm 1$ µs, $T^*_{2,2\uparrow} = 11.6 \pm 1$ µs. We assume that the noise follows a Gaussian distribution and we take

correlation terms $\langle \delta f_i \delta f_j \rangle \approx 0$. The variance of the fluctuations will follow the relation:

$$\begin{aligned} \langle \delta f^2_{\uparrow\downarrow} \rangle &= \frac{1}{2\pi^2 (T^*_{2,1\downarrow})^2} \\ \langle \delta f^2_{\uparrow\uparrow} \rangle + \langle \delta f^2_{\downarrow\uparrow} \rangle &= \frac{1}{2\pi^2 (T^*_{2,1\uparrow})^2} \\ \langle \delta f^2_{\downarrow\uparrow} \rangle &= \frac{1}{2\pi^2 (T^*_{2,2\downarrow})^2} \\ \langle \delta f^2_{\uparrow\uparrow} \rangle + \langle \delta f^2_{\uparrow\downarrow} \rangle &= \frac{1}{2\pi^2 (T^*_{2,2\uparrow})^2} \end{aligned} . \tag{9}$$

We obtain the standard deviation for three different fluctuations $\sigma_{f_{\uparrow\uparrow}} = \sqrt{\langle |\delta f_{\uparrow\uparrow}|^2 \rangle} = 16.1$ kHz, $\sigma_{f_{\uparrow\downarrow}} = \sqrt{\langle |\delta f_{\uparrow\downarrow}|^2 \rangle} = 10.1$ kHz, $\sigma_{f_{\downarrow\uparrow}} = \sqrt{\langle |\delta f_{\downarrow\uparrow}|^2 \rangle} = 21.0$ kHz. We perform time evolution simulation of the free induction decay measurement, which show that the $T_2^*$ values are consistent with our measurement, further corroborating that the correlating noise can be neglected when estimating the system fidelity. The effect of frequency fluctuations on the Clifford fidelity is plotted in Fig. S4. With quasi-static noise included in the model, the average Clifford fidelity is $F_{\text{Clifford}} = 97.5$ % in simulation which is 3 % points higher than the experimental result. Pulse calibration errors and power fluctuations of the microwave source are not included in this model and can realistically contribute 1-2 % points to the error.

---


[1] V. Srinivasa, K. C. Nowack, M. Shafiei, L. M. K. Vandersypen, and J. M. Taylor, Phys. Rev. Lett. **110**, 196803 (2013).

[2] C. Yang, A. Rossi, R. Ruskov, N. Lai, F. Mohiyaddin, S. Lee, C. Tahan, G. Klimeck, A. Morello, and A. Dzurak, Nature Communications **4**, 2069 (2013).

[3] T. Meunier, V. E. Calado, and L. M. K. Vandersypen, Phys. Rev. B **83**, 121403 (2011).

[4] M. Russ, D. M. Zajac, A. J. Sigillito, F. Borjans, J. M. Taylor, J. R. Petta, and G. Burkard, Phys. Rev. B **97**, 085421 (2018).

[5] D. C. McKay, C. J. Wood, S. Sheldon, J. M. Chow, and J. M. Gambetta, Phys. Rev. A **96**, 022330 (2017).

[6] M. Veldhorst, J. C. C. Hwang, C. H. Yang, A. W. Leenstra, B. de Ronde, J. P. Dehollain, J. T. Muhonen, F. E. Hudson, K. M. Itoh, A. Morello, and A. S. Dzurak, Nature Nanotechnology **9**, 981 (2014).

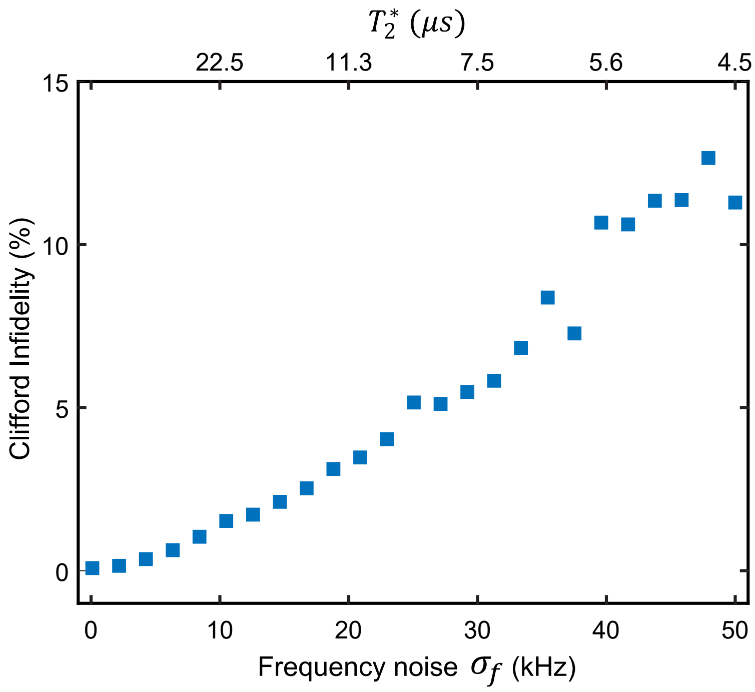


**Figure S4 | Clifford gate error as a function of standard deviation of quasi-static frequency noise** Simulation of the effect of frequency noise on the Clifford gate error. For simplicity, we keep the standard deviation of the frequency noise the same for all levels, $\sigma_f = \sigma_{f_{\uparrow\uparrow}} = \sigma_{f_{\uparrow\downarrow}} = \sigma_{f_{\uparrow\downarrow}}$. $F_{\text{Clifford}} > 99\%$ requires $T_2^* > 112$ µs on both qubit, which has been demonstrated before for Si quantum dots[6]. Our particular RB implementation is limited by $T_2^*$ as the qubits are idling for 50 % of the operation time. Simultaneously driving two qubits can reduce the idling time and extend the $T_2^*$ limit. Other remedies include faster gate operations, gates that possess dynamical decoupling properties, or optimized shaped pulses.
